# Supplementary material for: LUMINOUS: Indoor Scene Generation for Embodied AI Challenges
Source: arXiv:2111.05527 source file (2021-11-10)
Supplement: Supplementary file 1 [file _experimental_design_appendix.tex]

\section{Initial Experiment Plan}
experimental design for testing Luminous for embodied AI challenge
1. [Scene generation quality] Compare scene generation quality with other scene generation methods. (confusion score + user study)

2. [Task completion score] Test scenes based on supported Embodied AI task for different room layouts, report average test completion rate
3. [Task transfer rate] Test the success rate for transferring ALFRED challenge tasks to our env.

4. [ALFRED test score on transferred scenes] Test different SOTA methods on the minimal ALFRED challenge.
5. [ALFRED improvement] Test different SOTA methods trained on our data on the original ALFRED challenge.

6. [REARRANGEMENT]

\section{Scene Transfer Details}
This part describes the details for transferring tasks in ALFRED challenge to Luminous. The transfer process consists of several steps:
\begin{itemize}
    \item  \textbf{Scene information retrieval}: after getting a task in ALFRED, Luminous derives the information necessary for replicating the task including: scene type (kitchen, living room, bedroom and bathroom), 
\end{itemize}

Saved sections: 

\textbf{training data stats} [Yizhou 2]
\textbf{LUMINOUS evaluation} [Yizhou 1]

Advantage of EAI version: 
More efficient than ALFRED generation.

evaluation using EAI script to generate task and trajectories. 
\begin{itemize}
    \item four room types: each room type select 10 scenes, each scene use 25 trajectories. 4 x 10 x 25 = 1000
    \item  ET$\_$Human$\_$synth, Hitut, MOCA.
    \item  luminous valid seen [done] 
    \item  luminous valid unseen [todo] 
    \item  alfred valid seen  and unseen [todo] 
\end{itemize}

\begin{itemize}
    \item task type distribution: 
    \item Luminous room level distribution.
\end{itemize}

\textbf{LUMINOUS training and augmentation}[Yizhou 3]

\begin{itemize}
    \item Train ET and Hitut
    \item Luminous subgoal level distribution.
\end{itemize}

Scene quality evaluation.

back up results. 
\begin{table}[t]
\begin{tabular}{cc}
    \setlength{\aboverulesep}{0pt}
    \setlength{\belowrulesep}{0pt}
    \begin{small}
    \begin{tabular}{lar}
    & \mcc{2}{c}{\bf Task Success Rate} \\
    & \thor & \framework \\
    & (Human) & (Generated) \\
    \toprule
    Pick \& Place & .33 & .13 ($\Delta$-\bad{.20}) \\
    Pick Two \& Place & .10 & .06 ($\Delta$-\good{.04}) \\
    Examine in Light & .55 & .59 ($\Delta$\phantom{-}\good{.04}) \\
    Clean \& Place & .18 & .17 ($\Delta$-\good{.01}) \\
    Heat \& Place & .19 & .09 ($\Delta$-\bad{.10}) \\
    Cool \& Place & .07 & .07 ($\Delta$\phantom{-}\good{.00}) \\
    Stack \& Place & .05 & .09 ($\Delta$-\good{.04}) \\
    \midrule
    Overall & .21 & .17 ($\Delta$-\good{.04}) \\
    \bottomrule
    \end{tabular}
    \end{small}
    &
    \setlength{\aboverulesep}{0pt}
    \setlength{\belowrulesep}{0pt}
    \begin{small}
    \begin{tabular}{lar}
    & \mcc{2}{c}{\bf Subgoal statistics} \\
    & \thor & \framework \\
    & (Human) & (Generated) \\
    \toprule
    Heat Object & .021 & .010 ($\Delta$-\good{.011}) \\
    Cool Object & .009 & .007 ($\Delta$-\good{.002}) \\
    Clean Object & .018 & .018 ($\Delta$\phantom{-}\good{.000}) \\
    Slice Object & .008 & .007 ($\Delta$-\good{.001}) \\
    Put Object & .161 & .131 ($\Delta$-\good{.030}) \\
    Toggle Object & .067 & .109 ($\Delta$\phantom{-}\good{.042}) \\
    Pickup Object & .229 & .241 ($\Delta$\phantom{-}\good{.012}) \\
    Goto Location & .487 & .477 ($\Delta$-\good{.010}) \\
    \bottomrule
    \end{tabular}
    \end{small}
\end{tabular}
\caption{
\textbf{Left: Task Success Rate.} For most task types, the loss in success rate between \thor\ human-created scenes and \framework\ generated scenes is \good{less than 5\%}, and for some tasks success rate improves.
\textbf{Right: Subgoal Success Rate.} Multiple subgoals are carried out for each task.
The loss in success rate in \framework\ generated scenes is never \good{less than 5\%}, and sometimes improves.}
    \label{tab:task_sb_completion}
\end{table}
