# Supplementary material for: LUMINOUS: Indoor Scene Generation for Embodied AI Challenges
Source: arXiv:2111.05527 source file (2021-11-10)
Supplement: Supplementary file 2 [file appendix_exp.tex]

\newpage 
\section{Additional Experiments on User Study}

\begin{table}[h!tp]
\centering
\label{tab:user_study_app}
\begin{tabular}{|c|cc|cc|}
\hline
\multirow{2}{*}{Method} & \multicolumn{2}{c|}{Functionality}    & \multicolumn{2}{c|}{Naturalness} \\  \cline{2-5} 
                        & Bedroom        & Living room & Bedroom  & Living room   \\ \hline
AI2Thor               &   $4.23 \pm 0.97$ &  $3.97 \pm 1.14$   &    $3.68 \pm 1.07$  & $3.56 \pm 1.27$  \\
\framework                & $4.13 \pm 1.00$ & $3.28 \pm 1.40$ &  $3.83 \pm 1.11$    &   $2.87 \pm 1.47$      \\ \hline
Deep Priors                  & $2.43 \pm 1.41$  &  - &  $1.73 \pm 1.03$   &  -   \\ \hline
3D-SLN                  & $2.45 \pm 1.43$   &  -   &   $2.03 \pm 1.35$  &   -   \\ \hline
% Human-Centric                 &  &   &     &      \\ \hline
% SceneFormer                 &  &   &     &      \\ \hline
\end{tabular}\\
\caption{Human subjects' ratings (1-5) of generated scenes (without any post-process such as removing bad samples) in terms of Functionality and Naturalness.}
\end{table}

\section{Additional Experiments on Embodied Metrics}

\textbf{Embodied Metrics}: In this section, we introduce our evaluation on the generated scenes from the perspective of supporting Embodied AI tasks. We propose to measure the quality of scenes by the following embodied metrics:

\begin{itemize}[leftmargin=0.3in]
    \item Navigation Landmarks: we label important landmarks using objects in scenes and verify the robot can navigate to the those landmarks in the generated scenes. , we test our baseline on two types of indoor scenes 
    \item Navigation Routes: we define several routes using pairs of objects (e.g., Sofa to TV, Book to Floor Lamp) and verify whether the generated scene exists a navigable path between those pair of objects.
    \item Task completion: we design basic Embodied AI tasks in both living room and bed room and verify 
    whether the task can be successfully completed in the generated scene. 
\end{itemize}

% Please add the following required packages to your document preamble:
% \usepackage{multirow}

As the results shown in Table~\ref{tab:eval_embodied AI}, \framework\ can generate simulated environment that more than $94\%$ and $86\%$ of predefined landmarks in the scene are reachable in bedroom and living room, respectively.

\begin{table}[thbp]
\centering
\label{tab:eval_embodied AI}
\begin{tabular}{|c|cc|cc|cc|}
\hline
\multirow{2}{*}{Method} & \multicolumn{4}{c|}{Navigation Landmarks}  \\ \cline{2-5} 
                        & \multicolumn{2}{c|}{Bedroom}            & \multicolumn{2}{c|}{Living room}    \\ \hline
 AI2Thor                &    &      &          &           \\  \hline
\framework                &   $ 94.44\% \pm 0.11$   &  $74\%$      &        $86.63\% \pm 0.14 $   &  $40.43 \%$              \\  \hline
\end{tabular}\\
\caption{Embodied AI evaluations. The percentage in the first, third column denote average and standard deviation of the number of navigable landmarks across 50 generated scenes in Bedroom and Living room, respectively.  The percentage in the 
second, forth column denotes the percentage of scenes that all landmarks navigable.
}
\end{table}

New Task completion rate (June 14) Livingroom 84\% (42/50)\\
New Task completion rate (June 14) Bedroom 86\% (43/50)
