# Supplementary material for: LUMINOUS: Indoor Scene Generation for Embodied AI Challenges
Source: arXiv:2111.05527 source file (2021-11-10)
Supplement: Supplementary file 3 [file app_negative_socialimpact.tex]

\section{Potential Negative Societal Impact}
\label{sec:app:neg}
Our work focuses on facilitating the research in developing embodied learning agents with better generalization
performance to interact with a human through natural language under various indoor scenarios. The rapid development of embodied AI, robotics, and autonomous systems
reveals the great potential of building embodied agents that can follow humans' instructions to accomplish simple tasks. However, the safety regulations of embodied agents remain unexplored. We are deeply concerned by the possibility that our techniques might enable building robots to follow human
instructions without any safety restrictions. As researchers, we oppose any use or applications of our framework without rigorous investigation on the safety issue. It is our responsibility to emphasize that enforcing safety boundaries in embodied scenarios is significantly challenging. Fundamental AI research for embodied agents under safety constraints is imperative, especially with the ever-growing availability of autonomous devices or robots and their increasing capabilities.
