# Supplementary material for: LUMINOUS: Indoor Scene Generation for Embodied AI Challenges
Source: arXiv:2111.05527 source file (2021-11-10)
Supplement: Supplementary file 4 [file limitations.tex]

\section{Rewrite: Luminous for Alfred}
Can \framework\ benefit the training or testing for Embodied AI challenges? We answer this question by applying \framework\ for automatically generating additional data for \alfred\, a well-recognized challenge that requires manipulating the agent from multi-modalities, including images and language inputs.

Originally, \alfred\ collected the training and testing data by sampling tasks and corresponding task-solving trajectories through trials and errors from a Fast-Forward Planner (FF-Planner). The language instructions describing the agent's behaviors were annotated manually by humans. The inefficient process of task sampling (see Section 4.1) and the consuming human labeling make it hard to collect a large amount of data, which results in a mere number of $251$ tasks in $4$ scenes for validation and $255$ tasks in $8$ room for testing. 

We build a more efficient pipeline for automatically generating trajectories as training or testing data for \alfred\ based on \framework: task definitions are transferred from \alfred\ dataset instead of sampled from the FF-Planner; natural language instructions are synthesized instead of manually labeled. More importantly, incorporating CSSG and the task execution part in \framework\ , we can get an unlimited number of trajectories incurred in various room layouts.

In detail, given a trajectory $T_i$ from the \alfred\ training dataset, we employ a task parser to deduce objects and their relationships and save the scene conditions into the indoor-scene description part $I_i$ of CDF. Since each training scene in \alfred\ supports dozens of trajectories $\{T_i\}_{i=1,2,...}$, there may be some conflicting parts in their scene description $\{I_i\}_{i=1,2,...}$. For example, one task requires $\{Apple\_1\}$ to be on the countertop; another says $\{Apple\_1\}$ should be in the fridge. We propose a $merge$ operator $merge(I_1, I_2, ... ) \to \hat{I}$, where $\hat{I}$ denotes the merged links in indoor-scene description file, that tries to maximize common parts in the scene descriptions to tackle this problem. We use this merge operation for sampling indoor scene layouts $S$ by CSSG. Since \alfred\ does not change the positions of large pieces of furniture, such as fridges, sofas, and beds, the $merge$ operator records the requirements for large pieces of furniture and extracts the most common criteria for small objects (e.g., apple, cup, and book). Figure \ref{fig:images_comparison0} shows the comparison between \thor\ original scenes and \framework\ scenes generated to augment the \alfred\ challenge. 
After obtaining an indoor scene $S$, we apply two techniques to sample tasks and trajectories. The first follows the Fast-Forward Planner (FF-Planner)~\cite{shridhar2020alfred} and samples tasks and trajectories by sequentially setting initial conditions, sampling task goals, and executing trajectories. The second follows the original task design $D_i$ and directly applies the \textit{task execution} component to generate the trajectory $T'_i$. 
Locations of small objects defined by $I_i$ must be resampled for each task before execution.

The FF-Planner is slower at sampling tasks because it experiences trial and error in different sampling stages. We compare the efficiency of this method between sampling from \thor\ original scenes and from \framework-generated scenes in Section~\ref{sec:exp:scenequality}. The sampling efficiency indicates the quality of the indoor scene. The second method samples trajectories much faster since it directly applies the task design $D_i$ from original \alfred\ training data which can be quickly solved by the \textsc{Task execution} stage in \framework. We apply this method to generate a large number of scenes for the evaluation performance of different models in Section~\ref{sec:exp:eval}. 

\section{Additional limitations}
Another limitation is that \framework\ cannot self-justify that it can generate \alfred\ trajectories of the same quality as original ones, since the synthesized scenes sampled from CSSG may bring implicit biases to the distribution of object locations. The synthesized language may not be accurate enough compared well human annotations. Moreover, we have not figured out a strategy to make the synthesized trajectories helpful for training EAI models. 

Finally, the current \framework\ cannot organically bring different parts of EAI challenges together: we run each section individually, and the experience of running one section brings no insights for improving others. We hope that future study of \framework\ can make a closed loop that brings task design, trajectory sampling, training, and testing EAI models together: the task design module samples tasks according to the feedback of EAI testing results, and the training adapts to new tasks and challenges. In this way, \framework\ would be better applied to VR, AR, and real-world scenarios of human-robot interaction.
