# Supplementary material for: LUMINOUS: Indoor Scene Generation for Embodied AI Challenges
Source: arXiv:2111.05527 source file (2021-11-10)
Supplement: Supplementary file 5 [file checklist.tex]

%%%%%%%%%%%%%%%%%%%%%%%%%%%%%%%%%%%%%%%%%%%%%%%%%%%%%%%%%%%%
\section*{Checklist}

%%% BEGIN INSTRUCTIONS %%%
% The checklist follows the references.  Please
% read the checklist guidelines carefully for information on how to answer these
% questions.  For each question, change the default \answerTODO{} to \answerYes{},
% \answerNo{}, or \answerNA{}.  You are strongly encouraged to include a {\bf
% justification to your answer}, either by referencing the appropriate section of
% your paper or providing a brief inline description.  For example:
% \begin{itemize}
%   \item Did you include the license to the code and datasets? \answerYes{Our code is available at \url{https://github.com/amazon-research/indoor-scene-generation-eai}.}
%   \item Did you include the license to the code and datasets? \answerYes{The code and the data are proprietary.}
%   \item Did you include the license to the code and datasets? \answerNA{}
% \end{itemize}
% Please do not modify the questions and only use the provided macros for your
% answers.  Note that the Checklist section does not count towards the page
% limit.  In your paper, please delete this instructions block and only keep the
% Checklist section heading above along with the questions/answers below.
%%% END INSTRUCTIONS %%%

\begin{enumerate}

\item For all authors...
\begin{enumerate}
  \item Do the main claims made in the abstract and introduction accurately reflect the paper's contributions and scope?
    \answerYes{See Section~1.}
  \item Did you describe the limitations of your work?
    \answerYes{See Section~\ref{sec:con}.}
  \item Did you discuss any potential negative societal impacts of your work?
    \answerYes{See Appendix Section~\ref{sec:app:neg}}
  \item Have you read the ethics review guidelines and ensured that your paper conforms to them?
    \answerYes{Our main focus on evaluation existing works to ensure that current models and baselines are safe and robust.}
\end{enumerate}

\item If you are including theoretical results...
\begin{enumerate}
  \item Did you state the full set of assumptions of all theoretical results?
    \answerNA{}
	\item Did you include complete proofs of all theoretical results?
    \answerNA{}
\end{enumerate}

\item If you ran experiments...
\begin{enumerate}
  \item Did you include the code, data, and instructions needed to reproduce the main experimental results (either in the supplemental material or as a URL)?
    \answerYes{Our code is available at   \url{https://github.com/amazon-research/indoor-scene-generation-eai}.}
  \item Did you specify all the training details (e.g., data splits, hyperparameters, how they were chosen)?
    \answerYes{We run the evaluation and sampling by fixing the random seeds and the experiment parameters can be seen in the configuration file on the Github.}
	\item Did you report error bars (e.g., with respect to the random seed after running experiments multiple times)?
    \answerYes{}
	\item Did you include the total amount of compute and the type of resources used (e.g., type of GPUs, internal cluster, or cloud provider)?
    \answerNo{All the experiment can be performed on a regular desktop or laptop. Extensive computation resource is not required.}
\end{enumerate}

\item If you are using existing assets (e.g., code, data, models) or curating/releasing new assets...
\begin{enumerate}
  \item If your work uses existing assets, did you cite the creators?
    \answerYes{}
  \item Did you mention the license of the assets?
    \answerYes{We use Creative Commons public licenses for the code of this project, please refer to our Github repository.}
  \item Did you include any new assets either in the supplemental material or as a URL?
    \answerYes{We provide script to generate the pre-processed dataset.}
  \item Did you discuss whether and how consent was obtained from people whose data you're using/curating?
    \answerYes{See Section~\ref{sec:exp}.}
  \item Did you discuss whether the data you are using/curating contains personally identifiable information or offensive content?
  \answerNA{}
    % \answerNo{Our data does not contain personally identifiable information nor offensive content.}
\end{enumerate}

\item If you used crowdsourcing or conducted research with human subjects...
\begin{enumerate}
  \item Did you include the full text of instructions given to participants and screenshots, if applicable?
    \answerYes{We conducted user study on Amazon Turk. The participants were presented with details instructions with words and images.}
  \item Did you describe any potential participant risks, with links to Institutional Review Board (IRB) approvals, if applicable?
    \answerNA{}
  \item Did you include the estimated hourly wage paid to participants and the total amount spent on participant compensation?
    \answerNA{}
\end{enumerate}

\end{enumerate}

%%%%%%%%%%%%%%%%%%%%%%%%%%%%%%%%%%%%%%%%%%%%%%%%%%%%%%%%%%%%
